# Supplementary material for: Are Proactive Interventions for Reddit Communities Feasible?
Source: arXiv:2111.11019 source file (2021-11-22)
Supplement: Supplementary file 1 [file appendix.tex]

\appendix
\section{Case Study: {\subreddit{The\_Donald}}}\label{app:donald}

In this section, we focus specifically on understanding the evolution of
\subreddit{The\_Donald}. \Cref{fig:appendix:trump} shows the evolution of the
subreddit as captured by our hierarchical clustering of topic vectors.

\begin{figure*}[h!]
\includegraphics[width=\linewidth]{evolution-figs/Dendrogram3.png}
\caption{Dendrogram of a sample set of subreddits after applying by hierarchical clustering
  on topic vectors. Here we see how \subreddit{The\_Donald} evolved from a meme
  subreddit (labeled 0; nearest to \subreddit{TuberSim}) to a political
  subreddit (labeled months 1-7; nearest to \subreddit{Republican},
  \subreddit{enoughsandersspam}, and \subreddit{altright} before it was
  classified as hateful) to a hateful subreddit (labeled months 12-40; nearest
  to \subreddit{altright} when it was banned). \rnnote{@Maaz: Please add months
  to the labels on the X axis}}
\label{fig:appendix:trump}
\end{figure*}
